# Supplementary material for: A Topological Quantum Field Theory for Character Varieties of Non-orientable Surfaces
Source: arXiv:2009.12310 source file (2023-05-01)
Supplement: Supplementary file 1 [file appendix.tex]

\section*{Appendix}

Let $S$ be $\AA^n_\CC$ with coordinates $x_1, \ldots, x_n$. In this section we discuss an algorithm for computing the class of certain varieties $X$ over $S$ in $\K(\Var/S)$. We use the following notation. Let $F, G$ be finite subsets of $\CC[x_1, \ldots, x_n, V]$ with $V = \{ y_1, \ldots, y_m \}$ for some $m \ge 0$. Then we write $X(V, F, G)$ for the (reduced) subvariety of $\AA^m_S$ given by $f = 0$ for all $f \in F$ and $g \ne 0$ for all $g \in G$. For example,
\[ \SL_2(\CC) \times_\CC S = X(\{ a, b, c, d \}, \{ ad - bc - 1 \}, \varnothing) \quad \text{ and } \quad \GL_2(\CC) \times_\CC S = X(\{ a, b, c, d \}, \varnothing, \{ ad - bc \}) . \]

Now consider the following recursive algorithm.
\begin{algorithm}
    Let $X = X(V, F, G)$ be a variety over $S$ as above.
    \begin{enumerate}[1.]
        \item First simplify $F$ as follows:
        \begin{enumerate}[(a)]
            \item \label{step:groebner} Replace $F$ with the reduced Gr\"obner basis for $F$.
            \item If any $f$ in $F$ is of the form $f = y_i - u$ with $u \in \CC[x_1, \ldots, x_n, V - \{ y_i \}]$, then substitute $y_i$ with $u$ in each element of $F$, remove $y_i$ from $V$, and go to (a).
            \item \label{step:squarefree} Replace each $f$ in $F$ with its square-free part. If anything changed, go to (a).
        \end{enumerate}
        
        \item \label{step:reduce_modulo_F} Reduce each $g \in G$ modulo $F$.
        
        \item If $1 \in F$ or $0 \in G$, then $X = \varnothing$ and return $[X] = 0$.
        
        \item If $F = G = \varnothing$, then $X = \AA^k_S$ with $k = \# V$, and return $[X] = [ \AA^1_S ]^k$.
        
        \item If there exist partitions $V = V_1 \sqcup V_2, F = F_1 \sqcup F_2$ and $G = G_1 \sqcup G_2$ such that $V_1, V_2 \ne \varnothing$ and $F_i, G_i \subset \CC[x_1, \ldots, x_n, V_i]$, then $X = X_1 \times_S X_2$ where $X_i = X(V_i, F_i, G_i)$. Therefore, return $[X] = [X_1] \cdot [X_2]$.
        
        % ---
        % \item Check if result was previously stored already.
        % ---
        
        \item If any $f \in F$ is univariate in some $x \in \{ x_1, \ldots, x_n \} \cup V$, then write $f = (x - \alpha_1) \cdots (x - \alpha_k)$. For each $i = 1, \ldots, k$, let $X_i = X(V, F \cup \{ x - \alpha_i \}, G)$. Now return $[X] = \sum_{i = 1}^{k} [X_i]$.
        
        \item \label{step:check_product_equation} If any $f \in F$ factors as $f = uv$ with $u, v$ both not constant, then let $X_1 = X(V, F \cup \{ u \}, G)$ and $X_2 = X(V, F \cup \{ v \}, G \cup \{ u \})$, and return $[X] = [X_1] + [X_2]$.
        
        \item If any $f \in F$ is of the form $f = y_i u + v$ with $u, v \in \CC[x_1, \ldots, x_n, V - \{ y_i \}]$, then let $X_1 = X(V, F \cup \{ u, v \}, G)$ and $X_2 = X(V - \{ y_i \}, F_2, G_2)$ where $F_2$ (resp. $G_2$) contains all $f$ in $F$ (resp. in $G$) where $y_i$ is substituted with $-v / u$ and homogenized by multiplying by a suitable number of factors $u$. Now return $[X] = [X_1] + [X_2]$.
        
        \item If $G$ is non-empty, then take some $g \in G$ and let $X_1 = X(V, F, G - \{ g \})$ and $X_2 = X(V, F \cup \{ g \}, G - \{ g \})$. Return $[X] = [X_1] - [X_2]$.
        
        \item Create a new symbol that represents the class of $X$ in $\K(\Var/S)$. Return this symbol.
    \end{enumerate}
\end{algorithm}

An implementation of this algorithm in Python can be found at \cite{Vogel_Github}.

We give some remarks on this algorithm. First, note that steps \ref{step:groebner} and \ref{step:reduce_modulo_F} depend on a monomial order: we choose the \textit{degree reverse lexicographic order}. Secondly, the factorization done in step \ref{step:squarefree} to determine the square-free part of polynomials can be stored and reused in step \ref{step:check_product_equation} (and even in later computations). Finally, since the algorithm is heavily recursive, it happens that the same computations are done multiple times. Therefore, it is more efficient to store intermediate results: we store any result that comes from steps 6 -- 10, and check before step 6 if the computation has already been done before.
